# Supplementary material for: GLASS: Global to Local Attention for Scene-Text Spotting
Source: arXiv:2208.03364 source file (2022-08-05)
Supplement: Supplementary file 1 [file supp.tex]

% updated April 2002 by Antje Endemann
% Based on CVPR 07 and LNCS, with modifications by DAF, AZ and elle, 2008 and AA, 2010, and CC, 2011; TT, 2014; AAS, 2016; AAS, 2020; TH, 2022

\documentclass[runningheads]{llncs}
\usepackage{graphicx}
% DO NOT USE \usepackage{times}, it will be removed by typesetters
%\usepackage{times}

\usepackage{tikz}
\usepackage{comment}
\usepackage{amsmath,amssymb} % define this before the line numbering.
\usepackage{color}
\usepackage{orcidlink}

\usepackage{xr}
\usepackage{epsfig}
\usepackage{graphicx}
\usepackage{amsmath}
\usepackage{amssymb}
\usepackage{booktabs}
\usepackage{fnpct}
\usepackage{multirow}
% Support for easy cross-referencing
\usepackage[capitalize]{cleveref}
\crefname{section}{Sec.}{Secs.}
\Crefname{section}{Section}{Sections}
% \Crefname{table}{Table}{Tables}
% \crefname{table}{Table}{Tables}
% The "axessiblity" package can be found at: https://ctan.org/pkg/axessibility?lang=en
\usepackage[accsupp]{axessibility}  % Improves PDF readability for those with disabilities.

\input{chapters/macros}

% INITIAL SUBMISSION - The following two lines are NOT commented
% CAMERA READY - Comment OUT the following two lines
% \usepackage{ruler}
% \usepackage[width=122mm,left=12mm,paperwidth=146mm,height=193mm,top=12mm,paperheight=217mm]{geometry}

\begin{document}
% \renewcommand\thelinenumber{\color[rgb]{0.2,0.5,0.8}\normalfont\sffamily\scriptsize\arabic{linenumber}\color[rgb]{0,0,0}}
% \renewcommand\makeLineNumber {\hss\thelinenumber\ \hspace{6mm} \rlap{\hskip\textwidth\ \hspace{6.5mm}\thelinenumber}}
% \linenumbers
\pagestyle{headings}
\mainmatter
\def\ECCVSubNumber{1384}  % Insert your submission number here

\title{GLASS: Global to Local Attention for Scene-Text Spotting - Supplementary Material} % Replace with your title

% INITIAL SUBMISSION 
%\begin{comment}
% \titlerunning{ECCV-22 submission ID \ECCVSubNumber} 
% \authorrunning{ECCV-22 submission ID \ECCVSubNumber} 
% \author{Anonymous ECCV submission}
% \institute{Paper ID \ECCVSubNumber}
%\end{comment}
%******************

% CAMERA READY SUBMISSION
% \begin{comment}
\titlerunning{GLASS}
% If the paper title is too long for the running head, you can set
% an abbreviated paper title here
%
\author{Roi Ronen\inst{1}\thanks{Equal contribution. For correspondence: \email{tsiper@amazon.com}}\orcidlink{0000-0002-5235-480X} \and 
Shahar Tsiper\inst{2*} \and
Oron Anschel\inst{2}  \and \\
Inbal Lavi\inst{2} \and 
Amir Markovitz\inst{2} \and
R. Manmatha\inst{2}}
\authorrunning{R. Ronen et al.}
% First names are abbreviated in the running head.
% If there are more than two authors, 'et al.' is used.
%
\institute{Viterbi Faculty of Electrical \& Computer Eng., Technion, Haifa, Israel \and AWS AI Labs}
% \\  \email{tsiper@amazon.com}} 
%******************
\maketitle

\input{supplementary/supp_content}

\clearpage
% ---- Bibliography ----
%
% BibTeX users should specify bibliography style 'splncs04'.
% References will then be sorted and formatted in the correct style.
%
\bibliographystyle{splncs04}
\bibliography{egbib}
\end{document}
